# Supplementary material for: General Item Representation Learning for Cold-start Content Recommendations
Source: arXiv:2404.13808 source file (2024-04-22)
Supplement: Supplementary file 1 [file appendix.tex]

\appendix

\pagenumbering{roman}

\setcounter{table}{0}
\setcounter{figure}{0}

\clearpage
\section*{Appendix}

%------------------------------------

\section{Implementation Details}
\label{sec:appendix:impl}

\begin{table}
  \caption{Data and Model Hyper-parameters}
  \centering
  % \vspace{-0.3cm}
  {
  \small
  \begin{tabular}{ cl | ccc }
    \toprule
    Var & Definition & MovieLens & YahooMovie & Chosun News \\
    \midrule
    $C$ & Number of content attributes & 2 & 2 & 2 \\
    \midrule
    $c = 1$ & First content attributes & Video & Video & Image \\
    $H_1$ & Height of image & 224 & 224 & 224 \\
    $W_1$ & Width of image & 224 & 224 & 224 \\
    \midrule
    $c = 2$ & Second content attributes & Text (Synopsis) & Text (Synopsis) & Text (Article) \\
     & Language & English & English & Korean \\
    $|V|$ & Vocabulary size & 30,522 & 30,522 & 8,002 \\
    \midrule
    $d$ & User, item embedding size & \multicolumn{3}{c}{$\{32,64,128,256,512,1024,2048\}$} \\
    $D$ & Token embedding size & 192 & 192 & 192 \\
    $d'^{(1)}$ & Query, Key, Value size in visual Transformer & 512 & 512 & 512 \\
    $d'^{(2)}$ & Query, Key, Value size in text Transformer & 768 & 768 & 768 \\
    $F$ & Number of frames per clip & 32 & 32 & N/A \\
    $P$ & Image patch size & 16 & 16 & 16 \\
    $L^{(1)}$ & Number of visual Transformer blocks & 4 & 4 & 4 \\
    $L^{(2)}$ & Number of text Transformer blocks & 12 & 12 & 12 \\
    \bottomrule
  \end{tabular}}
  % \vspace{-0.3cm}
  \label{tab:hyperparams}
\end{table}
